# Supplementary material for: Learning Non-Parametric Basis Independent Models from Point Queries via Low-Rank Methods
Source: arXiv:1310.1826 source file (2016-06-06)
Supplement: Supplementary file 2 [file colt-appendix-tract.tex]

%--------------------------------------------------
% Appendix : Tractability results
%
\section{Tractability results}
